# Supplementary material for: Enabling Compute-Communication Overlap in Distributed Deep Learning Training Platforms
Source: arXiv:2007.00156 source file (2022-05-04)
Supplement: Supplementary file 1 [file appendix.tex]

\newpage
\section*{Appendix: Evaluations with Micro-benchmarks}

\insertFigureNew{topology}{Target Systems: 3D Torus and Fully-connected Switch Topology. Multiple NPU chips (M0-...) are connected within a package, and multiple packages (P0-...) are connected together, presenting heterogeneous scale-up bandwidth across the system. Connectivity is shown for NPU M0. NPU's M1/M2/M3 have similar connectivity - not shown}{0.9}

\begin{table}[h]
\caption{Topology details}
\label{tab:TopologyDetails}
\resizebox{\linewidth}{!}{%
\begin{tabular}{|l|l|l|}
\hline
\begin{tabular}[c]{@{}l@{}}Topology/\\ Dimension\\ Notation\end{tabular} &
  \begin{tabular}[c]{@{}l@{}}Collective\\ Algorithm\end{tabular} &
  BW/Dimension \\ \hline
\begin{tabular}[c]{@{}l@{}}3D torus /\\ L x V x H \\ (L is the \# of\\ NPUs within \\ a package, V\\ is the \#of\\ inter-package\\ rows, H is the\#\\ of inter-package\\ columns)\end{tabular} &
  \begin{tabular}[c]{@{}l@{}}Hierarchical all-reduce:\\ 1. Ring-based reduce-scatter in L\\ 2. Ring-based all-reduce in V\\ 3. Ring-based all-reduce in H\\ 4. Ring-based all-gather in L\\ \\ Hierarchical all-to-all:\\ 1. Ring-based all-to-all in L\\ 2. Ring-based all-to-all in V\\ 3. Ring-based all-to-all in H\end{tabular} &
  \begin{tabular}[c]{@{}l@{}}1 bi-directionl ring in L\\ (using 2 intra-packag\\ links/NPU),\\ 1 bi-directionl ring in V\\ (using 2 inter-packag\\ links/NPU),\\ 1 bi-directional ring in H\\ (using 2 inter-package\\ links/NPU)\\ \textbf{NOTE: If V/L=1, then}\\ \textbf{L/V has 2 bi-directional}\\  \textbf{rings.}\end{tabular} \\ \hline
\begin{tabular}[c]{@{}l@{}}Alltoall/\\ L x P\\ (L is the \#\\ of NPUs within\\ a package, P is\\ the \# of packages)\end{tabular} &
  \begin{tabular}[c]{@{}l@{}}Hierarchical all-reduce:\\ 1. Ring-based reduce-scatter in L\\ 2. Direct all-reduce in P\\ 3. Ring-based all-gather in L\\ \\ Hierarchical all-to-all:\\ 1. Ring-based all-to-all in L\\ 2. Direct all-to-all in P\end{tabular} &
  \begin{tabular}[c]{@{}l@{}}1 bidirectional ring in L\\ (using 2 intra-package\\ links/NPU ),\\ 4 fully connected \\ switches (using\\ 4 inter-package\\ links/NPU )\end{tabular} \\ \hline
\end{tabular}%
}
\end{table}

\insertFigureNew{t_allreduce}{Baseline, \ncu and Ideal total communication latency ($\mu$s) of the all-reduce collective for the torus topology.}{0.9}

\insertFigureNew{t_alltoall}{Baseline, \ncu and Ideal total communication latency ($\mu$s) of the all-to-all collective for the torus topology.}{0.9}

\insertFigureNew{a2a_allreduce}{Baseline, \ncu and Ideal total communication latency  ($\mu$s) of the all-reduce collective for the alltoall topology.}{0.9}

\insertFigureNew{a2a_alltoall}{Baseline, \ncu and Ideal total communication latency ($\mu$s) of the all-to-all collective for the alltoall topology}{0.9}

\insertWideFigureNew{t_allreduce_detailed}{The detailed latency breakdown for all-reduce on torus network. The \textbf{NIC-NPU/Mem-NIC bus queuing} and \textbf{bus transfer} shows the average queening and average transfer time of transfer requests in NIC-NPU/Mem-NIC bus, respectively. The \textbf{local reduction} delay refers to the average latency of messages being reduced by the NPU. \textbf{Chunk queuing} is the average amount of time chunks are waiting for the chunks that are ahead of them to be finished and then start executing. \textbf{Message network transfer} refers to the average amount of time messages spend in the network.}{0.9}

In this Appendix, we present the performance of baseline, \ncu and Ideal for single all-reduce and all-to-all collectives. All-reduce is the only collective communication operation in most of the training workloads. However, sometimes all-to-all is used especially for recommendation model DNNs where all-to-all is used for embeddings.
\autoref{fig:topology} shows the two classes of topology and \autoref{tab:TopologyDetails} provides details of the hierarchical collective implementation.

%In \autoref{sec:results}, \autoref{fig:t_allreduce} presented the runtime of a single all-reduce on the torus topology. On average, using \ncu improves the total communication latency by 1.51$\times$ compared to the baseline.

\autoref{fig:t_allreduce} presents the runtime for running the all-reduce collective by itself. On average, using \ncu improves the total communication latency by 1.51$\times$ compared to the baseline. Ideal is only 1.43$\times$ better than \ncu, while compared to baseline, Ideal is 2.17$\times$ better.

We observe a similar behavior with other collectives and systems.  \autoref{fig:t_alltoall}, \autoref{fig:a2a_allreduce}, and  \autoref{fig:a2a_alltoall} show the performance of the three systems for all-to-all on torus, all-reduce on alltoall, and all-to-all on alltoall, respectively. On average \ncu improves all-to-all on torus by 1.22$\times$, all-reduce on alltoall by 1.55$\times$ and all-to-all on alltoall by 1.20$\times$, compared to the baseline system.

To delve deeper into the reason of this improvement,  \autoref{fig:t_allreduce_detailed} shows the detailed time breakdown for \autoref{fig:t_allreduce}. As shown in the figure, due to better performance, the average chunk queuing is  reduced by 44.9\% on average in \ncu compared to the baseline. In addition, \ncu significantly reduces the bus congestion (total NIC-NPU/Mem-NIC bus queuing + transfer) by 88.9\% on average compared to the baseline. Note that in general  the message network transfer in \ncu is smaller than baseline/ideal systems because in \ncu, chunk sizes (and hence message sizes) are smaller because of the limited on-chip SRAM. However, as \autoref{fig:t_allreduce_detailed} and \autoref{fig:t_allreduce} show, this limitation does not prevent \ncu from driving the network in a much more efficient way compared to the baseline.
