# Supplementary material for: Enabling Compute-Communication Overlap in Distributed Deep Learning Training Platforms
Source: arXiv:2007.00156 source file (2022-05-04)
Supplement: Supplementary file 2 [file appendix-bgwork.tex]

\insertFigureNew{CollectiveOperations2}{Overview of collective communication operation used in DNN training networks.}{0.7}
